# Supplementary material for: Thermal (and Hybrid Thermal/Audio) Side-Channel Attacks on Keyboard Input
Source: arXiv:2210.02234 source file (2022-10-05)
Supplement: Supplementary file 1 [file 10-appendix.tex]

\section{Comparison with Similar Attacks}
\label{sec:compare}
We now compare \attack with several similar human factors-based 
insider attacks. We focus on several aspects: adversary's \emph{Goal}, any \emph{Required Equipment}, the 
\emph{Timeliness} requirements, whether a \emph{Careless Victim} is needed, and finally, if \emph{Prior Profiling} of the
victim is required. Summary of the comparison is shown in Table \ref{tab:comp}.

\begin{table*}[th!]
	\caption{\small{Feature Comparison of Common Human-Based Attack Types.}}
	\label{tab:comp}
	\centering
	\begin{tabular}{|c||c|c|c|c|c|c|}
		\hline\cline{1-6}
		Attack              &     Attack                &   Adversary &  Careless  & Equipment & Prior Profiling
		\\
		Type:               &     Goal:                 &    Timeliness       &   Victim?    & Needed:  & Required?
		\\ \hline \cline{1-6}
		\lunch              &     Hijack  &     $15$ min (default)                  &   YES        & None & NO
		\\ & Log-in Session  & & & \\ \hline
		\surf                 &     Password          &    Real-Time                 &   YES        & Pair of Eyes  & NO
		\\ & & & & or Video Camera&
		\\ \hline
		\acoust            &     Password          &    Real-Time                &   NO          & Audio & YES
		\\ & & & & Recorder&
		\\ \hline
		\vibrat              &     Password          &     Real-Time               &   NO          & Accelerometer & YES
		\\ \hline
		\attack             &     Password          &     up to $1$ min                  &   NO          & Thermal & NO
		\\ & & & & Camera&
		\\ \hline \cline{1-6}
	\end{tabular}
\end{table*}

\subsection{\lunch}
\luncha are performed by the insider adversary who relies on a careless victim that neglects to terminate 
their secure log-in session \cite{shamir1999playing}. 
\begin{compactitem}
	\item \emph{Objective}: to gain access to a single secure (authenticated) session.
	\item \emph{Required Equipment}: none, the adversary only needs to physically access the computer once the victim leaves. 
	\item \emph{Timeliness:} determined by the de-authentication technique(s) used by the victim. For example, the default inactivity
	timeout for Windows machines is a generous $15$ minutes. 
	\item \emph{Careless Victim}: required for this attack to work. At the minimum, the victim needs to leave their 
	workstation unattended without logging out or locking the screen.
	\item \emph{Profiling}: no prior victim profiling is needed. The adversary can be opportunistic; it gains access to an 
	authenticated session with out any additional or prior knowledge required.
\end{compactitem}

\subsection{\surf}
\surfa are performed by the insider adversary who looks over the shoulder of a careless victim while the password is entered.
It can also be performed with the aid of a (perhaps hidden) camera pointed at the victim's keyboard, in which case adversarial
presence is not required.
\begin{compactitem}
	\item \emph{Objective}: to learn the victim's password. 
	\item \emph{Required Equipment}: none, though a video camera can be useful.
	\item \emph{Timeliness}  real-time, as the adversary must watch victim password entry as it occurs.
	\item \emph{Careless Victim}: required, since the adversary has to stand over the victim's terminal to
	watch them type in their password. Careless victim is not required in case of a pre-placed viceoa camera.
	\item \emph{Profiling}: no prior victim profiling is needed and the adversary can be opportunistic: it learns the 
	victim's password with no additional or prior knowledge.
\end{compactitem}

\subsection{\acoust}
\acousta are performed by the insider adversary who instruments the victim's environment with an audio 
recording device and exploits acoustic dynamics \cite{zhuang2009keyboard}
\begin{compactitem}
	\item \emph{Objective}: learn the victim's password. 
	\item \emph{Required Equipment}: an audio recording device, placed nearby.
	\item \emph{Timeliness}: real-time, since the adversary must record the keyboard sounds instantaneously.
	\item \emph{Careless Victim}: not required; the recording device can be hidden from view.
	\item \emph{Profiling}: prior victim profiling is needed; the adversary must build an acoustic profile 
	of the victim to accurately interpret keystroke sounds.
\end{compactitem}

\subsection{\vibrat}
\vibrata are performed by the insider adversary using an accelerometer to record vibrations created by a victim 
typing into a keyboard, in order to reconstruct what was typed \cite{marquardt2011sp}.
\begin{compactitem}
	\item \emph{Objective}: learn the victim's password. 
	\item \emph{Required Equipment}: an accelerometer, placed nearby (closer than in \acousta).
	\item \emph{Timeliness}: real-time, since the adversary must record the victim's vibrations instantaneously.
	\item \emph{Careless Victim}: not required; the recording device can be hidden from view. 
	\item \emph{Profiling}: prior victim profiling is needed; the adversary must build a vibration profile  in order
	to accurately interpret keystroke vibration patterns.
\end{compactitem}

\subsection{\attack}
\attacka are performed by an insider adversary who records thermal residues users after recent password entry.
\begin{compactitem}
	\item \emph{Objective}: learn the victim's password. 
	\item \emph{Required Equipment}: thermal camera.
	\item \emph{Timeliness}: up to $1$ minute, the adversary must record the keyboard before thermal residues dissipate.
	\item \emph{Careless Victim}: not required; recording/imaging takes place after the victim leaves.
	\item \emph{Profiling}: prior victim profiling not needed. The adversary does not need any prior knowledge of the victim
	to analyze thermal images (though it obviously helps, especially with insecure passwords).
\end{compactitem}
